# Supplementary material for: Part-aware Unified Representation of Language and Skeleton for Zero-shot Action Recognition
Source: arXiv:2406.13327 source file (2024-06-19)
Supplement: Supplementary file 1 [file X_suppl.tex]

\clearpage
\setcounter{page}{1}
\setcounter{section}{0}
\setcounter{table}{0}
\setcounter{figure}{0}
\maketitlesupplementary

% \textcolor{red}{
In this supplementary material, we present additional information to explain and support our design choices and their concrete effects in each methodology module of PURLS. Additionally,
% }
we list the remaining experiment performance that we omitted in the main paper and provide a qualitative visualization of the learning outcome of our solution.

\section{Additional Information for Local Semantic Divison}
PURLS aligns local visual semantics with global/body-part-based/temporal-interval-based descriptions against a given label. %To reduce calculation costs, we individually consider spatially and temporally local semantics. 
In the submission, we meticulously analyze the spatial and temporal local semantics when they are respectively extracted, resulting in a total of $P + Z + 1$ aligned representations.  Alternatively, if we jointly consider spatial-temporal semantics,  there will be  $P * Z + 1$  aligned representations (\ie finding temporal local movements for each spatial local area).  To streamline computational costs, we opt for the approach of separately considering spatial and temporal local semantics.   %Specifically, we set the total number of aligned representations as $P + Z + 1$ instead of $P * Z + 1$ (\ie separating temporal movements for each spatially local area). 

\begin{table*}[ht]
\centering
\resizebox{.8\textwidth}{!}{%
\begin{tabular}{|c|c|}
\hline
\textbf{Description Type} & \textbf{Questions}            \\ \hline
\multirow{5}{*}{Body-part-based} &
  \begin{tabular}[c]{@{}c@{}}Using the following format, describe in very short \textbf{how each body part moves} \\ \textbf{/ how a person's body part would act / individual body part action} for \textless{}Action\textgreater{}.\end{tabular} \\ \cline{2-2} 
                          & Head would: \textit{\{text\}}          \\ \cline{2-2} 
                          & Hands would: \textit{\{text\}}         \\ \cline{2-2} 
                          & Torso would: \textit{\{text\}}         \\ \cline{2-2} 
                          & Legs would: \textit{\{text\} }         \\ \hline
\multirow{4}{*}{Temporal-interval-based} &
  \begin{tabular}[c]{@{}c@{}}Use the following format, separate in very short \textbf{how a person performs the} \\ \textbf{action of / the motion of / the sub-motions when a person carries} \\ \textbf{out} \textless{}Action\textgreater into three phases.\end{tabular} \\ \cline{2-2} 
                          & 1: The person would \textit{\{text\}}. \\ \cline{2-2} 
                          & 2: The person would \textit{\{text\}}. \\ \cline{2-2} 
                          & 3: The person would \textit{\{text\}}. \\ \hline
\multirow{2}{*}{Global} &
  \begin{tabular}[c]{@{}c@{}}Using the following format, describe in very short \textbf{the motion of a person who / the motion}\\  \textbf{of a person carries out / how a person does} \textless{}Action\textgreater.\end{tabular} \\ \cline{2-2} 
                          & The person would \textit{\{text\}}.    \\ \hline
\end{tabular}%
}
\caption{The full version of the designed questions used to generate label-relative descriptions under different scales. The bold texts represent the question alternatives, while \textit{\{text\}} refers to the blanks for GPT-3 to fill.}
\label{Table: prompt-select}
\end{table*}
\begin{table*}[ht]
\centering
\resizebox{.9\textwidth}{!}{%
\begin{tabular}{cccccccccc}
\toprule
\multirow{2}{*}{\textbf{\#   Prompt question}} &
  \multirow{2}{*}{\textbf{\# Description per question}} &
  \multicolumn{4}{c}{\textbf{NTU-RGBD 60 (Acc \%)}} &
  \multicolumn{4}{c}{\textbf{NTU-RGBD 120 (Acc \%)}} \\
  &    & 55/5  & 48/12 & 40/20 & 30/30 & 110/10 & 96/24 & 80/40 & 60/60 \\ \midrule
1 & 1  & \textbf{79.23} & 40.99 & \textbf{31.05} & 23.52 & \textbf{71.95}  & \textbf{52.01} & \textbf{28.38} & \textbf{19.63} \\
2 & 1  & 75.44 & \textbf{45.64} & 26.38 & \textbf{24.72} & 61.87  & 45.28 & 25.10  & 15.76 \\
3 & 1  & 76.90 & 43.63 & 26.37 & 24.67 & 63.00  & 43.96 & 25.01 & 15.73 \\
1 & 5  & 78.50     & 41.57     & 27.25     & 22.02     & 67.59      & 44.06     & 26.32     & 16.39     \\
1 & 10 & 77.7  & 41.99 & 27.01 & 22.33 & 66.51  & 44.60 & 26.56 & 16.96 \\ \bottomrule
\end{tabular}%
}
\caption{Hyperparameter ablation (\%) of applying different numbers of prompt questions \& generated descriptions on GPT-3. `\# Prompt question' refers to the number of used questions. `\# Desc per question' means the number of generated descriptions for each question.}
\label{Table: q_prompt}
\end{table*}
\begin{table*}[ht]
\centering
\resizebox{.7\textwidth}{!}{%
\begin{tabular}{|c|c|}
\hline
{\color[HTML]{333333} \textbf{Description Type}} & {\color[HTML]{333333} \textbf{Prompts}}                                                                       \\ \hline
{\color[HTML]{333333} }                          & {\color[HTML]{333333} A cropped video of people's head motions that   \textless{}Description\textgreater{}.}  \\ \cline{2-2} 
{\color[HTML]{333333} }                          & {\color[HTML]{333333} A cropped video of people's   hand motions that \textless{}Description\textgreater{}.}  \\ \cline{2-2} 
{\color[HTML]{333333} }                          & {\color[HTML]{333333} A cropped video of people's torso motions   that \textless{}Description\textgreater{}.} \\ \cline{2-2} 
\multirow{-4}{*}{{\color[HTML]{333333} Body-part-based}} &
  {\color[HTML]{333333} A cropped video of people's leg motions   that \textless{}Description\textgreater{}.} \\ \hline
{\color[HTML]{333333} Temporal-interval-based} &
  {\color[HTML]{333333} A trimmed video of the motion that \textless{}Description\textgreater{}.} \\ \hline
{\color[HTML]{333333} Global}           & {\color[HTML]{333333} A video of people's motion that \textless{}Description\textgreater{}.}                  \\ \hline
\end{tabular}%
}
\caption{The customized prompts used to wrap each description before it is sent to CLIP. }
\label{Table: clip-prompt}
\end{table*}

\section{Additional Information for Creating Description-based Text Features}
The descriptions for each label from every evaluation dataset are provided in the supplement repository under the path of `supplement/gpt3\_desc.xlsx'. 
% \textcolor{red}{
For body-part-based local movements, we generated descriptions for four body areas including `Head', `Hands', `Torso', and `Legs'. For temporal-interval-based local movements, we generated descriptions for three phases including `Start', `Middle', and `End'. A manual inspection was applied to ensure that all descriptions properly enhance the original label semantics.
% }

\subsection{Hyperparameter selection for generating descriptions}
In the main submission, we used only one question and one generated answer for each description type when preparing the text encoding inputs for CLIP. Meanwhile, we also attempted to use varying numbers of questions and answers to check their influence on the model performance. 
% \textcolor{red}{
In \cref{Table: prompt-select}, we present the wrapping prompts for each global/local part and all the alternative questions we designed for each type of description generation (see the design explanation in \cref{subsec: desc} of our main paper). \cref{Table: q_prompt} records the hyperparameter ablation when we use different numbers of questions and answers for the generation. When multiple descriptions are generated, we respectively encode each answer and average all output features to calculate the linguistic embeddings later used for semantic alignments.
% }
Yet, unlike traditional supervised learning, we observed that including multiple questions and answers does not improve ZSL classification in most cases. Therefore, we only use one question and one answer for each description in our main experiments.

\subsection{Preprocessing for CLIP inputs}
A pre-trained text encoder from CLIP 
% \cite{clip} 
requires proper prompting on its input to ensure the backbone outputs fit the required downstream tasks. Hence, as shown in \cref{Table: clip-prompt}, we prepared customized prompting sentences to further standardize each generated description before encoding them.

% TODO
\section{Additional Information for Adaptive Partitioning}
\begin{table}[]
\centering
\resizebox{\columnwidth}{!}{%
\begin{tabular}{lccccccccc} \toprule
\multicolumn{1}{c}{\multirow{2}{*}{\textbf{BP}}} &
  \multirow{2}{*}{\textbf{TI}} &
  \multicolumn{4}{c}{\textbf{NTU-RGBD 60 (Acc \%)}} &
  \multicolumn{4}{c}{\textbf{NTU-RGBD 120 (Acc \%)}} \\
\multicolumn{1}{c}{} &   & 55/5           & 48/12          & 40/20          & 30/30          & 110/10         & 96/24          & 80/40          & 60/60          \\ \midrule
1                    & 3 & 77.70          & 40.69          & 28.84          & 22.46          & 71.26          & 46.13          & 24.43          & 18.57          \\
2                    & 3 & 78.31          & 33.15          & 30.81          & 23.03          & 72.77          & 45.90          & 26.26          & \textbf{19.65} \\
4                    & 3 & \textbf{79.23} & \textbf{40.99} & \textbf{31.05} & \textbf{23.52} & \textbf{71.95} & \textbf{52.01} & \textbf{28.38} & 19.63          \\
6                    & 3 & 72.18          & 37.65          & 30.10          & 23.35          & 62.67          & 47.81          & 26.39          & 18.78          \\
4                    & 1 & 76.32          & 37.62          & 29.06          & 21.91          & 71.73          & 40.92          & 23.49          & 19.13          \\
4                    & 3 & \textbf{79.23} & \textbf{40.99} & \textbf{31.05} & \textbf{23.52} & \textbf{71.95} & \textbf{52.01} & \textbf{28.38} & 19.63          \\
4                    & 6 & 74.54          & 38.89          & 28.70          & 23.03          & 71.00          & 48.81          & 26.11          & 17.71    \\ \bottomrule     
\end{tabular}%
}
\caption{Hyperparameter ablation (\%) on \textit{NTU-RGB+D 60} and \textit{NTU-RGB+D 120} of (1) using different numbers of body-part-based (BP) local partitioning, (2) using different numbers of temporal-interval-based (TI) local partitioning.}
\label{Table: local}
\end{table}
\subsection{Hyperparameter selection for Local Representations}
In the main submission, we choose to align local movements using four body-part-based (BP) partitions and three temporal-interval-based (TI) partitions (\ie $P = 4$, $Z = 3$). \cref{Table: local} provides the hyperparameter ablation when we try different numbers of spatial/temporal local representations. In the case of BP, using one body part means directly calculating the global features along the spatial dimension. Using two body parts refers to splitting spatial features into upper and lower body movements. Using six body parts requires further decomposing hand and leg movements into individual single-hand and single-leg movements. In the case of TI, the original sequence is averagely divided into multiple time intervals according to the specified number. The results reveal that having four body parts and three temporal intervals yields the best performance for PURLS.

\subsection{Visualization for Adaptive Partitioning}
\cref{fig:att-h}, \cref{fig:att-full}, \cref{fig:att-l}, and \cref{fig:att-r} visualize the learned weights for acquiring the corresponding visual representations towards the descriptions for the classes `apply cream on face', `running on the spot', `kicking other person', and `cutting nails'. We analyze the impacts of adaptive partitioning in four scenarios. 
Two spatial-based scenarios include learning the actions characterized by specific local body movements (\eg `applying cream on face') or the movement from the entire body (\eg `running on the spot'). Two temporal-based scenarios include learning the actions that can be broken down into sequentially local movements (\eg `kicking other person'), and the actions that involve repetitive movements (\eg `cutting nails'). To showcase the different learning focus in a more intuitive manner, we demonstrate the respective feature sampling weight of each body joint on every temporal dimension.

\begin{figure*}[ht]
  \centering
   \includegraphics[width=\textwidth]{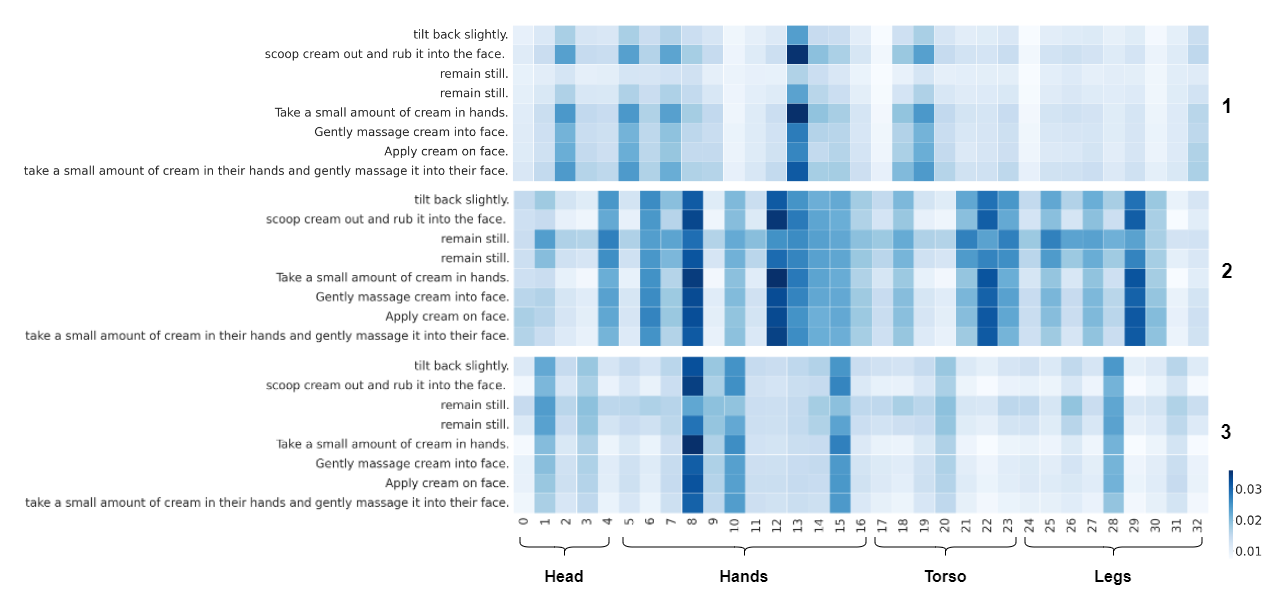}

   \caption{Visualized illustration of the learned adaptive weights used for sampling joint features to generate the visual representation of each description on `apply cream on face'. The horizontal axis lists each body joint, and the vertical axis is the convoluted temporal dimension with a length of $L'$. We trunk the temporal dimension into three groups for the phases of `start' (1), `middle' (2), and `end' (3). And we label the default body part that each body joint usually belongs to according to \cref{fig:pt} in our main paper. For the demonstration in one phase, from top to bottom is the feature weight distribution against the description for body-part-based (`head', `hands', `torso', `legs'), temporal-interval-base (`start', `middle', `end'), and global semantics. }
   \label{fig:att-h}
\end{figure*}

\begin{figure*}[ht]
  \centering
   \includegraphics[width=\textwidth]{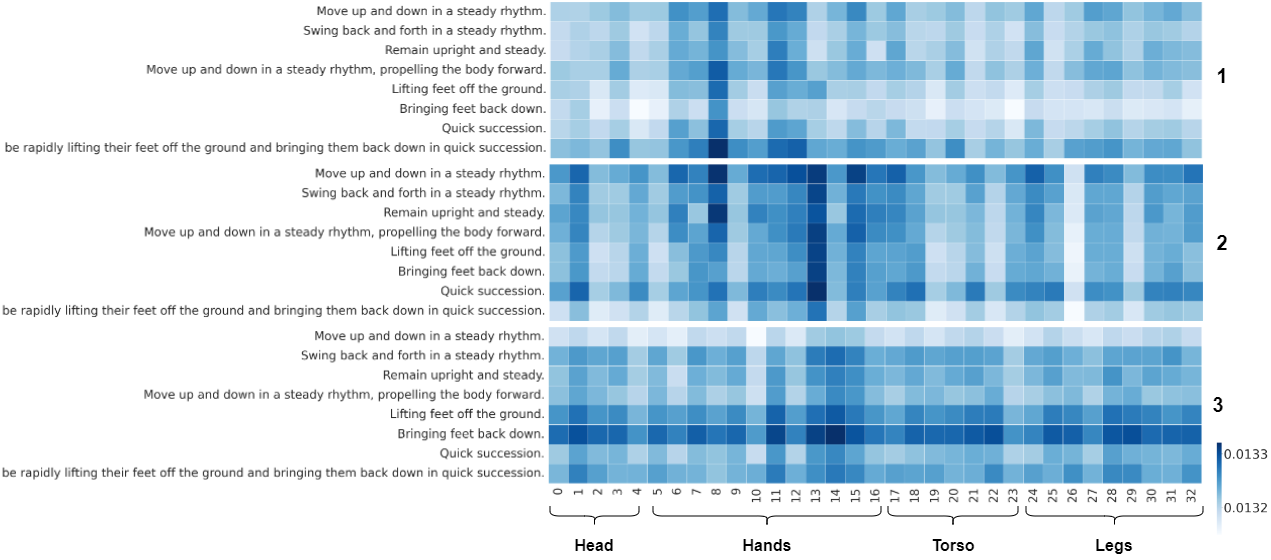}

   \caption{Visualized illustration of the learned adaptive weights for the class `running on the spot'.}
   \label{fig:att-full}
\end{figure*}

\begin{figure*}[ht]
  \centering
   \includegraphics[width=\textwidth]{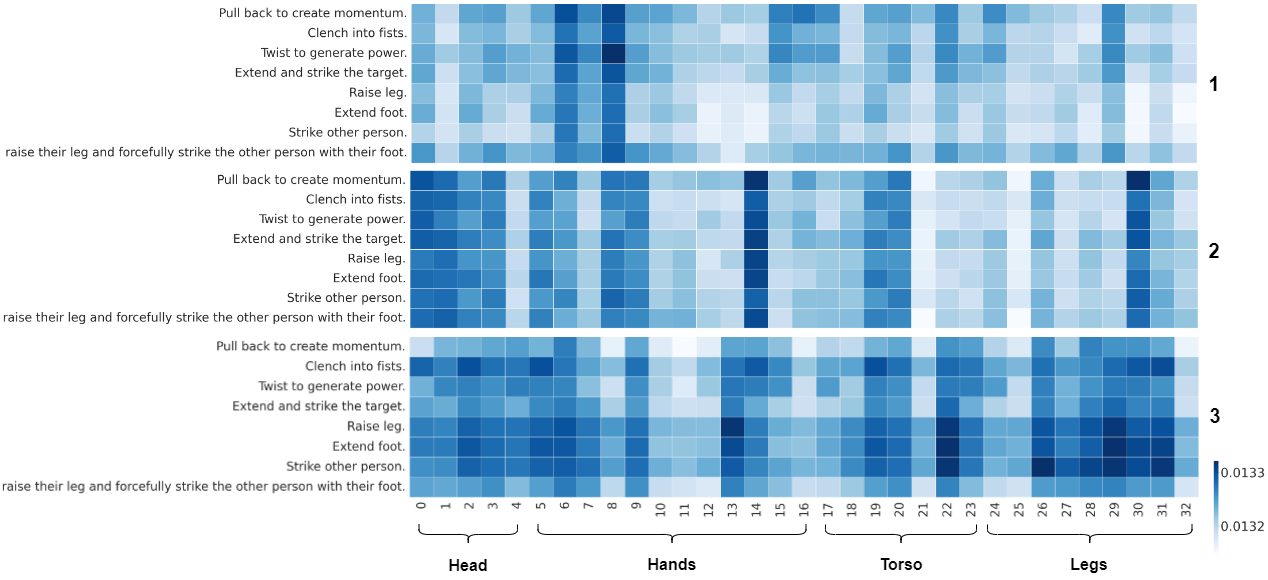}

   \caption{Visualized illustration of the learned adaptive weights for the class `kicking other person'.}
   \label{fig:att-l}
\end{figure*}

\begin{figure*}[ht]
  \centering
   \includegraphics[width=\textwidth]{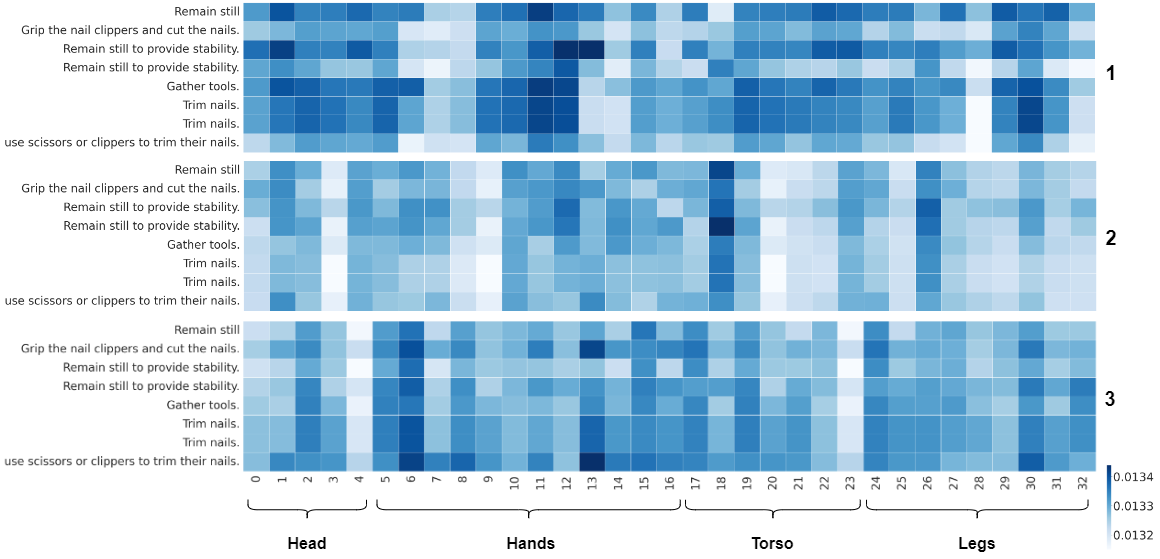}

   \caption{Visualized illustration of the learned adaptive weights for the class `cutting nails'.}
   \label{fig:att-r}
\end{figure*}

    \textbf{Adaptive partioning for spatially local movements}: For the actions characterized by specific local body movements (\cref{fig:att-h}),  against body-part-based descriptions (Row 1-4 in each phase), adaptive partitioning effectively highlights the feature sampling from the body joints belonging to the `hands'. It also assigns contextual significance to a few body-joint features from the `torso' and `legs' during the middle phase, as some co-movements may exist when raising arms to one's face. The local representation of hand movements emphasizes these features the most. The representations for other descriptions learn each joint feature in a more averaged manner while still giving the most importance to hand features, as they become the most valuable context features.  Against the actions characterized by the entire body movement (\cref{fig:att-full}), we find the module more averagely samples the body-joint-level features for each description.  

\textbf{Adaptive partioning for temporally local movements}: For the actions that can be broken down into sequentially local movements (\cref{fig:att-l}), against temporal-interval-based descriptions (Row 5-7 in each phase), adaptive partitioning emphasizes the overall features in the third phase, which contains the most representative postures of the kicking movement. The representation for the `end' phase assigns the highest weights to these features to represent its local description as `Strike other person.' Meanwhile, multiple hand-related features are collected with higher priority in the first two phases, while some leg-related features are also collected in the second phase. This implies that PURLS also allocates attention to sampling the hand and leg movements for representing the descriptions of `Raise leg' and `Extend foot'. Against the actions that repeat temporally local movements (\cref{fig:att-r}), we observe a relatively balanced distribution of learning focus. In particular, the distribution tends to concentrate slightly more in the first phase. We believe this is because most relevant visual information is already available at the beginning. On the other hand, the ending phase may contain noises from the zero-padding frames.

\section{Additional Information for Experiments}
% NTU 60 chart
\begin{figure}[ht]
\centering
\resizebox{.85\columnwidth}{!}{
\begin{tikzpicture}
\begin{axis}[
    xlabel=\# Unseen Classes, 
    ylabel=Accuracy (\%), 
    xtick={5, 12, 20, 30},
    tick align=inside,
    legend style={font=\fontsize{8}{8}\selectfont},
    legend pos=north east,
    ymajorgrids=true,
    grid style=dashed
    ]

\addplot[sharp plot,mark=square,green] plot coordinates {
    (5, 75.37)
    (12, 26.44)
    (20, 24.26)
    (30, 14.81)
};
\addlegendentry{ReViSE}

\addplot[sharp plot,mark=square,blue] plot coordinates {
    (5, 77.61)
    (12, 35.8)
    (20, 26.91)
    (30, 18.45)
};
\addlegendentry{DeViSE}

\addplot[sharp plot,mark=square,red] plot coordinates {
    (5, 64.39)
    (12, 24.67)
    (20, 20.05)
    (30, 12.39)
};
\addlegendentry{JPoSE}

\addplot[sharp plot,mark=square,gray] plot coordinates {
    (5, 62.71)
    (12, 24.73)
    (20, 16.21)
    (30, 11.51)
};
\addlegendentry{CADA-VAE}

\addplot[sharp plot,mark=square,brown] plot coordinates {
    (5, 58.33)
    (12, 28.35)
    (20, 19.85)
    (30, 12.00)
};
\addlegendentry{SynSE}
\addplot[sharp plot,mark=square,orange] plot coordinates {
    (5, 64.69)
    (12, 35.46)
    (20, 27.15)
    (30, 16.29)
};
\addlegendentry{Global}
\addplot[sharp plot,mark=square,black] plot coordinates {
    (5, 79.23)
    (12, 40.99)
    (20, 31.05)
    (30, 23.52)
};
\addlegendentry{PURLS}
\end{axis}
\end{tikzpicture}
}
\caption{Visualized accuracy variation on \textit{NTU-RGB+D 60}.}
\label{fig:ntu60-v}
\end{figure}

% NTU 120 chart
\begin{figure}[ht]
\centering
\resizebox{.85\columnwidth}{!}{
\begin{tikzpicture}
\begin{axis}[
    xlabel=\# Unseen Classes, 
    ylabel=Accuracy (\%), 
    xtick={10, 24, 40, 60},
    tick align=inside,
    legend style={font=\fontsize{8}{8}\selectfont},
    legend pos=north east,
    ymajorgrids=true,
    grid style=dashed
    ]

\addplot[sharp plot,mark=square,green] plot coordinates {
    (10, 57.92)
    (24, 37.96)
    (40, 19.47)
    (60, 8.27)
};
\addlegendentry{ReViSE}

\addplot[sharp plot,mark=square,blue] plot coordinates {
    (10, 61.52)
    (24, 40.91)
    (40, 19.5)
    (60, 12.19)
};
\addlegendentry{DeViSE}

\addplot[sharp plot,mark=square,red] plot coordinates {
    (10, 49.54)
    (24, 33.42)
    (40, 13.71)
    (60, 7.65)
};
\addlegendentry{JPoSE}

\addplot[sharp plot,mark=square,gray] plot coordinates {
    (10, 46.67)
    (24, 20.49)
    (40, 10.55)
    (60, 5.67)
};
\addlegendentry{CADA-VAE}

\addplot[sharp plot,mark=square,brown] plot coordinates {
    (10, 46.91)
    (24, 28.03)
    (40, 13.64)
    (60, 7.73)
};
\addlegendentry{SynSE}
\addplot[sharp plot,mark=square,orange] plot coordinates {
    (10, 66.96)
    (24, 44.27)
    (40, 21.31)
    (60, 14.12)
};
\addlegendentry{Global}
\addplot[sharp plot,mark=square,black] plot coordinates {
    (10, 71.95)
    (24, 52.01)
    (40, 28.38)
    (60, 19.63)
};
\addlegendentry{PURLS}
\end{axis}
\end{tikzpicture}
}
\caption{Visualized accuracy variation on \textit{NTU-RGB+D 120}.}
\label{fig:ntu120-v}
\end{figure}

% Kinetic chart
\begin{figure}[ht]
\centering
\resizebox{.85\columnwidth}{!}{
\begin{tikzpicture}
\begin{axis}[
    xlabel=\# Unseen Classes, 
    ylabel=Accuracy (\%), 
    xtick={20, 40, 60, 80},
    tick align=inside,
    legend style={font=\fontsize{8}{8}\selectfont},
    legend pos=north east,
    ymajorgrids=true,
    grid style=dashed
    ]

\addplot[sharp plot,mark=square,green] plot coordinates {
    (20, 24.95)
    (40, 13.28)
    (60, 8.14)
    (80, 6.23)
};
\addlegendentry{ReViSE}

\addplot[sharp plot,mark=square,blue] plot coordinates {
    (20, 22.22)
    (40, 12.32)
    (60, 7.97)
    (80, 5.65)
};
\addlegendentry{DeViSE}

\addplot[sharp plot,mark=square,orange] plot coordinates {
    (20, 25.96)
    (40, 15.85)
    (60, 10.23)
    (80, 7.77)
};
\addlegendentry{Global}
\addplot[sharp plot,mark=square,black] plot coordinates {
    (20, 32.22)
    (40, 22.56)
    (60, 12.02)
    (80, 11.75)
};
\addlegendentry{PURLS}
\end{axis}
\end{tikzpicture}
}
\caption{Visualized accuracy variation on \textit{Kinetics-skeleton 200}.}
\label{fig:kinetic-v}
\end{figure}

\begin{figure}[ht]
\centering
\resizebox{.85\columnwidth}{!}{
\begin{tikzpicture}
\begin{axis}[
    xlabel=\# Unseen Classes, 
    ylabel=Accuracy (\%), 
    xtick={40, 80, 100, 120},
    tick align=inside,
    legend style={font=\fontsize{8}{8}\selectfont},
    legend pos=north east,
    ymajorgrids=true,
    grid style=dashed
    ]

\addplot[sharp plot,mark=square,green] plot coordinates {
    (40, 20.84)
    (80, 11.82)
    (100, 9.49)
    (120, 8.23)
};
\addlegendentry{ReViSE}

\addplot[sharp plot,mark=square,blue] plot coordinates {
    (40, 18.37)
    (80, 10.23)
    (100, 9.47)
    (120, 8.34)
};
\addlegendentry{DeViSE}

\addplot[sharp plot,mark=square,orange] plot coordinates {
    (40, 22.50)
    (80, 15.08)
    (100, 11.44)
    (120, 11.03)
};
\addlegendentry{Global}
\addplot[sharp plot,mark=square,black] plot coordinates {
    (40, 34.51)
    (80, 24.32)
    (100, 16.99)
    (120, 14.28)
};
\addlegendentry{PURLS}
\end{axis}
\end{tikzpicture}
}
\caption{Visualized accuracy variation on \textit{Kinetics-skeleton 400}.}
\label{fig:kinetic400-v}
\end{figure}

\subsection{Seen/unseen Split Setups}
The specific lists of seen/unseen classes in each experiment split are provided as numpy files in the supplement repository under the path of `supplement/label\_splits'. Each split setting belongs to one of the following dataset folders: `ntu60', `ntu120', `kinetic200', `kinetic400', `nw-ucla', `utd-mhad', `uwa3dii'. The first three datasets are the ones we focus on in the main paper. For a given split, the file that contains the corresponding unseen class list is named as `ru + the number of unseen classes'. Similarly, the file recording the corresponding seen classes is named as `rs + the number of seen classes'. For example, for the split with 55 seen classes and 5 unseen classes on the \textit{NTU-RGB+D 60} dataset, the corresponding seen and unseen class lists are recorded in the files of `supplement/label\_splits/ntu60/rs55.npy' and `supplement/label\_splits/ntu60/ru5.npy'.

\subsection{Extra Visualization for Experiment Results}
\cref{fig:ntu60-v}, \cref{fig:ntu120-v} and \cref{fig:kinetic-v} visualize the accuracy gaps and changing curves of every baseline and PURLS when predicting different numbers of unseen classes on \textit{NTU-RGB+D 60}, \textit{NTU-RGB+D 120}, \textit{Kinetic-skeletons 200}. Our method reaches state-of-the-art prediction accuracies in every experimental setting. The performance conclusion on each dataset is consistent with the analysis in \cref{subsec: results} of our main paper. 

\subsection{Full Ablation Results}
\cref{table:ablation-supp1} and \cref{table:ablation-supp2} add extra results for the experiment setups we used for ablation study (see \cref{subsec: ablation} of our main paper) on the \textit{Kinetic-skeletons 200} dataset. 
\begin{table*}[ht]
\centering
\resizebox{\textwidth}{!}{%
\begin{tabular}{ccccccccccccc}
\toprule
 &
  \multicolumn{4}{c}{\textbf{NTU-RGBD 60 (Acc \%)}} &
  \multicolumn{4}{c}{\textbf{NTU-RGBD 120 (Acc \%)}} &
  \multicolumn{4}{c}{\textbf{Kinetic 200 (Acc \%)}} \\
\multirow{-2}{*}{\textbf{Partitioning   Strategy}} &
  55/5 &
  48/12 &
  40/20 &
  30/30 &
  110/10 &
  96/24 &
  80/40 &
  60/60 &
  180/20 &
  160/40 &
  140/60 &
  120/80 \\ \midrule
Global (Original) &
  64.69 &
  35.46 &
  27.15 &
  16.29 &
  66.96 &
  44.27 &
  21.31 &
  14.12 &
  25.96 &
  15.85 &
  10.23 &
  7.77 \\
Global (GPT-3) &
  {\color[HTML]{333333} 78.50} &
  33.47 &
  29.21 &
  22.27 &
  64.89 &
  47.15 &
  25.16 &
  17.46 &
  24.44 &
  14.08 &
  8.31 &
  7.06 \\
Static Partitioning &
  76.46 &
  33.03 &
  29.57 &
  22.00 &
  67.62 &
  46.83 &
  26.98 &
  18.03 &
  24.04 &
  15.60 &
  8.14 &
  7.74 \\
Adaptive Partitioning &
  \textbf{79.23} &
  \textbf{36.77} &
  \textbf{31.05} &
  \textbf{23.52} &
  \textbf{71.95} &
  \textbf{52.01} &
  \textbf{28.38} &
  \textbf{19.63} &
  \textbf{32.22} &
  \textbf{22.56} &
  \textbf{12.01} &
  \textbf{11.75} \\ \bottomrule
\end{tabular}%
}
\caption{Full ablation study (\%) on \textit{NTU-RGB+D 60}, \textit{NTU-RGB+D 120}, and \textit{Kinetics-skeleton 200} for using different alignment learning with partitioning strategies, including direct global feature alignment to label or global description semantics, and PURLS with static/adaptive partitioning.}
\label{table:ablation-supp1}
\end{table*}

\begin{table*}[ht]
\centering
\resizebox{\textwidth}{!}{%
\begin{threeparttable}
\begin{tabular}{cllcccccccccccc}
\toprule
\multirow{2}{*}{$\bm{\alpha_i}$} &
  \multicolumn{1}{c}{\multirow{2}{*}{\textbf{BP}}} &
  \multicolumn{1}{c}{\multirow{2}{*}{\textbf{TI}}} &
  \multicolumn{4}{c}{\textbf{NTU-RGBD 60 (Acc \%)}} &
  \multicolumn{4}{c}{\textbf{NTU-RGBD 120 (Acc \%)}} &
  \multicolumn{4}{c}{\textbf{Kinetic 200 (Acc \%)}} \\ 
 &
  \multicolumn{1}{c}{} &
  \multicolumn{1}{c}{} &
  55/5 &
  48/12 &
  40/20 &
  30/30 &
  110/10 &
  96/24 &
  80/40 &
  60/60 &
  180/20 &
  160/40 &
  140/60 &
  120/80 \\ \midrule
-  &  &  & 78.50 & 33.47 & 29.21 & 22.27 & 64.89     & 47.15    & 25.16    & 17.46 & 24.44 &
  14.08 &
  8.31 &
  7.06        \\ \midrule 
% Learnable &  &  & 66.15 & 33.03          & 22.38 & 16.50 & 40.55 & 33.56 & 16.49 & 10.84          \\ \midrule 
Average &\checkmark  &  & 76.68 & 37.80          & 30.92 & 22.20 & 68.11 & 30.93 & 24.36 & 18.67 & 22.32 & 7.12 & 3.63 & 5.60 \\ 
Learnable &\checkmark  &  & 76.32 & 37.62          & 29.06 & 21.91 & 71.73 & 40.92 & 23.49 & 19.13 & 22.73 & 14.79 & 8.24 & 7.69         \\ \midrule 
Average &  & \checkmark & 78.65 & 38.80 & 28.14 & 22.69 & 55.73 & 50.67 & 27.50 & 17.50 & 21.81 & 20.04 & 8.61 & 6.81         \\ 
Learnable &  & \checkmark & 77.70 & 40.69          & 28.84 & 22.46 & 71.26 & 46.13 & 24.43 & 18.57 & 24.85 & 18.73 & 7.97 & 7.95         \\ \midrule 
Average & \checkmark & \checkmark & 79.02 & 39.92          & 31.00 & 23.47 & \textbf{73.55} & 51.38 & 27.67 & 18.66        & 26.87 & 21.10 & 10.03 & 11.55  \\ 
Learnable & \checkmark
   & \checkmark   &
  \textbf{79.23} &
  \textbf{40.99} &
  \textbf{31.05} &
  \textbf{23.52} &
  71.95 &
  \textbf{52.01} &
  \textbf{28.38} &
  \textbf{19.63} &
  \textbf{32.22} &
  \textbf{22.56} &
  \textbf{12.01} &
  \textbf{11.75}\\ \bottomrule
\end{tabular}%
  \end{threeparttable}
}
\caption{Full ablation study (\%) on \textit{NTU-RGB+D 60}, \textit{NTU-RGB+D 120} and \text{Kinetics-skeleton 200} for (1) using different $\alpha_i$ ($i\in[0, P+Z+1)$) to sum for $L_{train}$, (2) adding body-part-based (BP) alignment learning, (3) adding temporal-interval-based (TI) alignment learning.}
\label{table:ablation-supp2}
\end{table*}

% \label{sec:rationale}
% % 
% Having the supplementary compiled together with the main paper means that:
% % 
% \begin{itemize}
% \item The supplementary can back-reference sections of the main paper, for example, we can refer to \cref{sec:intro};
% \item The main paper can forward reference sub-sections within the supplementary explicitly (e.g. referring to a particular experiment); 
% \item When submitted to arXiv, the supplementary will already included at the end of the paper.
% \end{itemize}
% % 
% To split the supplementary pages from the main paper, you can use \href{https://support.apple.com/en-ca/guide/preview/prvw11793/mac#:~:text=Delete%20a%20page%20from%20a,or%20choose%20Edit%20%3E%20Delete).}{Preview (on macOS)}, \href{https://www.adobe.com/acrobat/how-to/delete-pages-from-pdf.html#:~:text=Choose%20%E2%80%9CTools%E2%80%9D%20%3E%20%E2%80%9COrganize,or%20pages%20from%20the%20file.}{Adobe Acrobat} (on all OSs), as well as \href{https://superuser.com/questions/517986/is-it-possible-to-delete-some-pages-of-a-pdf-document}{command line tools}.

\subsection{Other Experiment Results}
\label{subsec: other results}
\textbf{\textit{Kinetic-skeleton 400}}: We provide \cref{Table: k400} to record the performance results of ReViSE, DeViSE, Global, and PURLS on \textit{Kinetics-skeleton 400} (See the dataset description in \cref{subsec: datasets} of our main paper). \cref{fig:kinetic400-v} visualizes the accuracy gaps and changing curves of every baseline and PURLS. We created four splits of $360/40$, $320/80$, $300/100$, and $280/120$ for evaluation. These setups are replaced with a similar but simpler testing protocol on \textit{Kinetics-skeleton 200}.

% Kinetic 400
\begin{table}[]
\centering
\resizebox{.8\columnwidth}{!}{%
\begin{tabular}{ccccc} \toprule
\multirow{2}{*}{\textbf{Model}}         & \multicolumn{4}{c}{\textbf{Kinetic 400 (Acc \%)}} \\
                                        & 360/40     & 320/80     & 300/100    & 280/120    \\ \midrule
ReViSE  & 20.84      & 11.82          & 9.49          & 8.23          \\
DeViSE  & 18.37      & 10.23          & 9.47          & 8.34          \\
Global                                  & 22.50      & 15.08          & 11.44          & 11.03          \\
PURLS                                   & \textbf{34.51}      & \textbf{24.32}          & \textbf{16.99}          & \textbf{14.28}         \\ \bottomrule
\end{tabular}%
}
\caption{Zero-shot action recognition results (\%) on \textit{Kinetics-skeleton 400} for PURLS \& all available baselines introduced in \cref{subsec: implementation} of our main paper.}
\label{Table: k400}
\end{table}

% \textcolor{red}{
\textbf{\textit{Small-scale datasets}}: \cref{Table: smalldataset} records the performance of ReViSE, DeViSE, Global, and PURLS on multiple small-scale datasets, including \textit{NW-UCLA}, \textit{UTD-MHAD}, and \textit{UWA3D II} (respectively containing 10, 27 and 10 common daily action classes). As shown in the table, PURLS also outperforms other baselines in these testing environments where a minimal semantic overlap between seen and unseen classes makes zero-shot recognition more challenging. 
% }

% Small datasets
\begin{table}[]
\centering
\resizebox{.9\columnwidth}{!}{%
\begin{threeparttable}
\setlength{\tabcolsep}{2pt} % Adjust the column separation here
\begin{tabular}{@{}ccccccccc@{}}
\toprule
\multirow{2}{*}{\textbf{Model}} & \multicolumn{2}{c}{\textbf{NW-UCLA}} & \multicolumn{3}{c}{\textbf{UTD-MHAD}} & \multicolumn{3}{c}{\textbf{UWA3D II}}\\
       & 8/2 & 5/5 & 22/5 & 18/9 & 14/13 & 24/6 & 20/10 & 15/15 \\ \midrule
ReViSE &  69.12   & 44.99    &  29.37    &  19.86    &  12.26  &  30.33    & 10.91     &  10.43   \\
DeViSE &  72.81   &  36.02   &  12.50    &  13.59    &  13.94  & 34.16     &  12.51    & 11.41    \\
Global &  73.49   &  46.83   &  23.00    &  18.47    &  14.38  &  32.18    &  15.63    &  11.02   \\ \midrule
PURLS  &  \textbf{75.84}   &  \textbf{49.47}   &  \textbf{57.50}    & \textbf{31.71}     &  \textbf{19.23} &  \textbf{35.65}    & \textbf{18.91}     &  \textbf{13.98}   \\ \bottomrule
\end{tabular}
\end{threeparttable}}
\caption{Zero-shot action recognition results (\%) on NW-UCLA, UTD-MHAD and UWA3D II for PURLS \& all available baselines.}
\label{Table: smalldataset}
\end{table}
